# Supplementary material for: Modeling Thousands of Human Annotators for Generalizable Text-to-Image Person Re-identification
Source: arXiv:2503.09962 source file (2025-03-13)
Supplement: Supplementary file 1 [file X_suppl.tex]

\clearpage
\setcounter{page}{1}
\maketitlesupplementary

This supplementary material includes five sections. Section \ref{sec:QwenInstruction} illustrates the instruction we use in Qwen2.5-7B to remove discriminative words in pedestrian descriptions. Section \ref{sec:Hyper} conducts ablation study on the value of some hyper-parameters in our method. The SDM loss \cite{jiang2023cross} used in ReID model training is introduced in Section \ref{sec:sdm}. In Section \ref{sec:ablation}, we provide more details about the ablation experiment in Section 4.3, including the extraction of the descriptive templates in the experiment (3) in Table 1 and the detailed setting of DBSCAN \cite{ester1996density} clustering in the experiment (7). Section \ref{sec:visualize} shows our MLLM-generated captions of the pedestrian images, which demonstrates the effectiveness of our method in simulating various human descriptive styles.

\begin{figure*}[tp]
  \centerline{\includegraphics[width=1.0\linewidth]{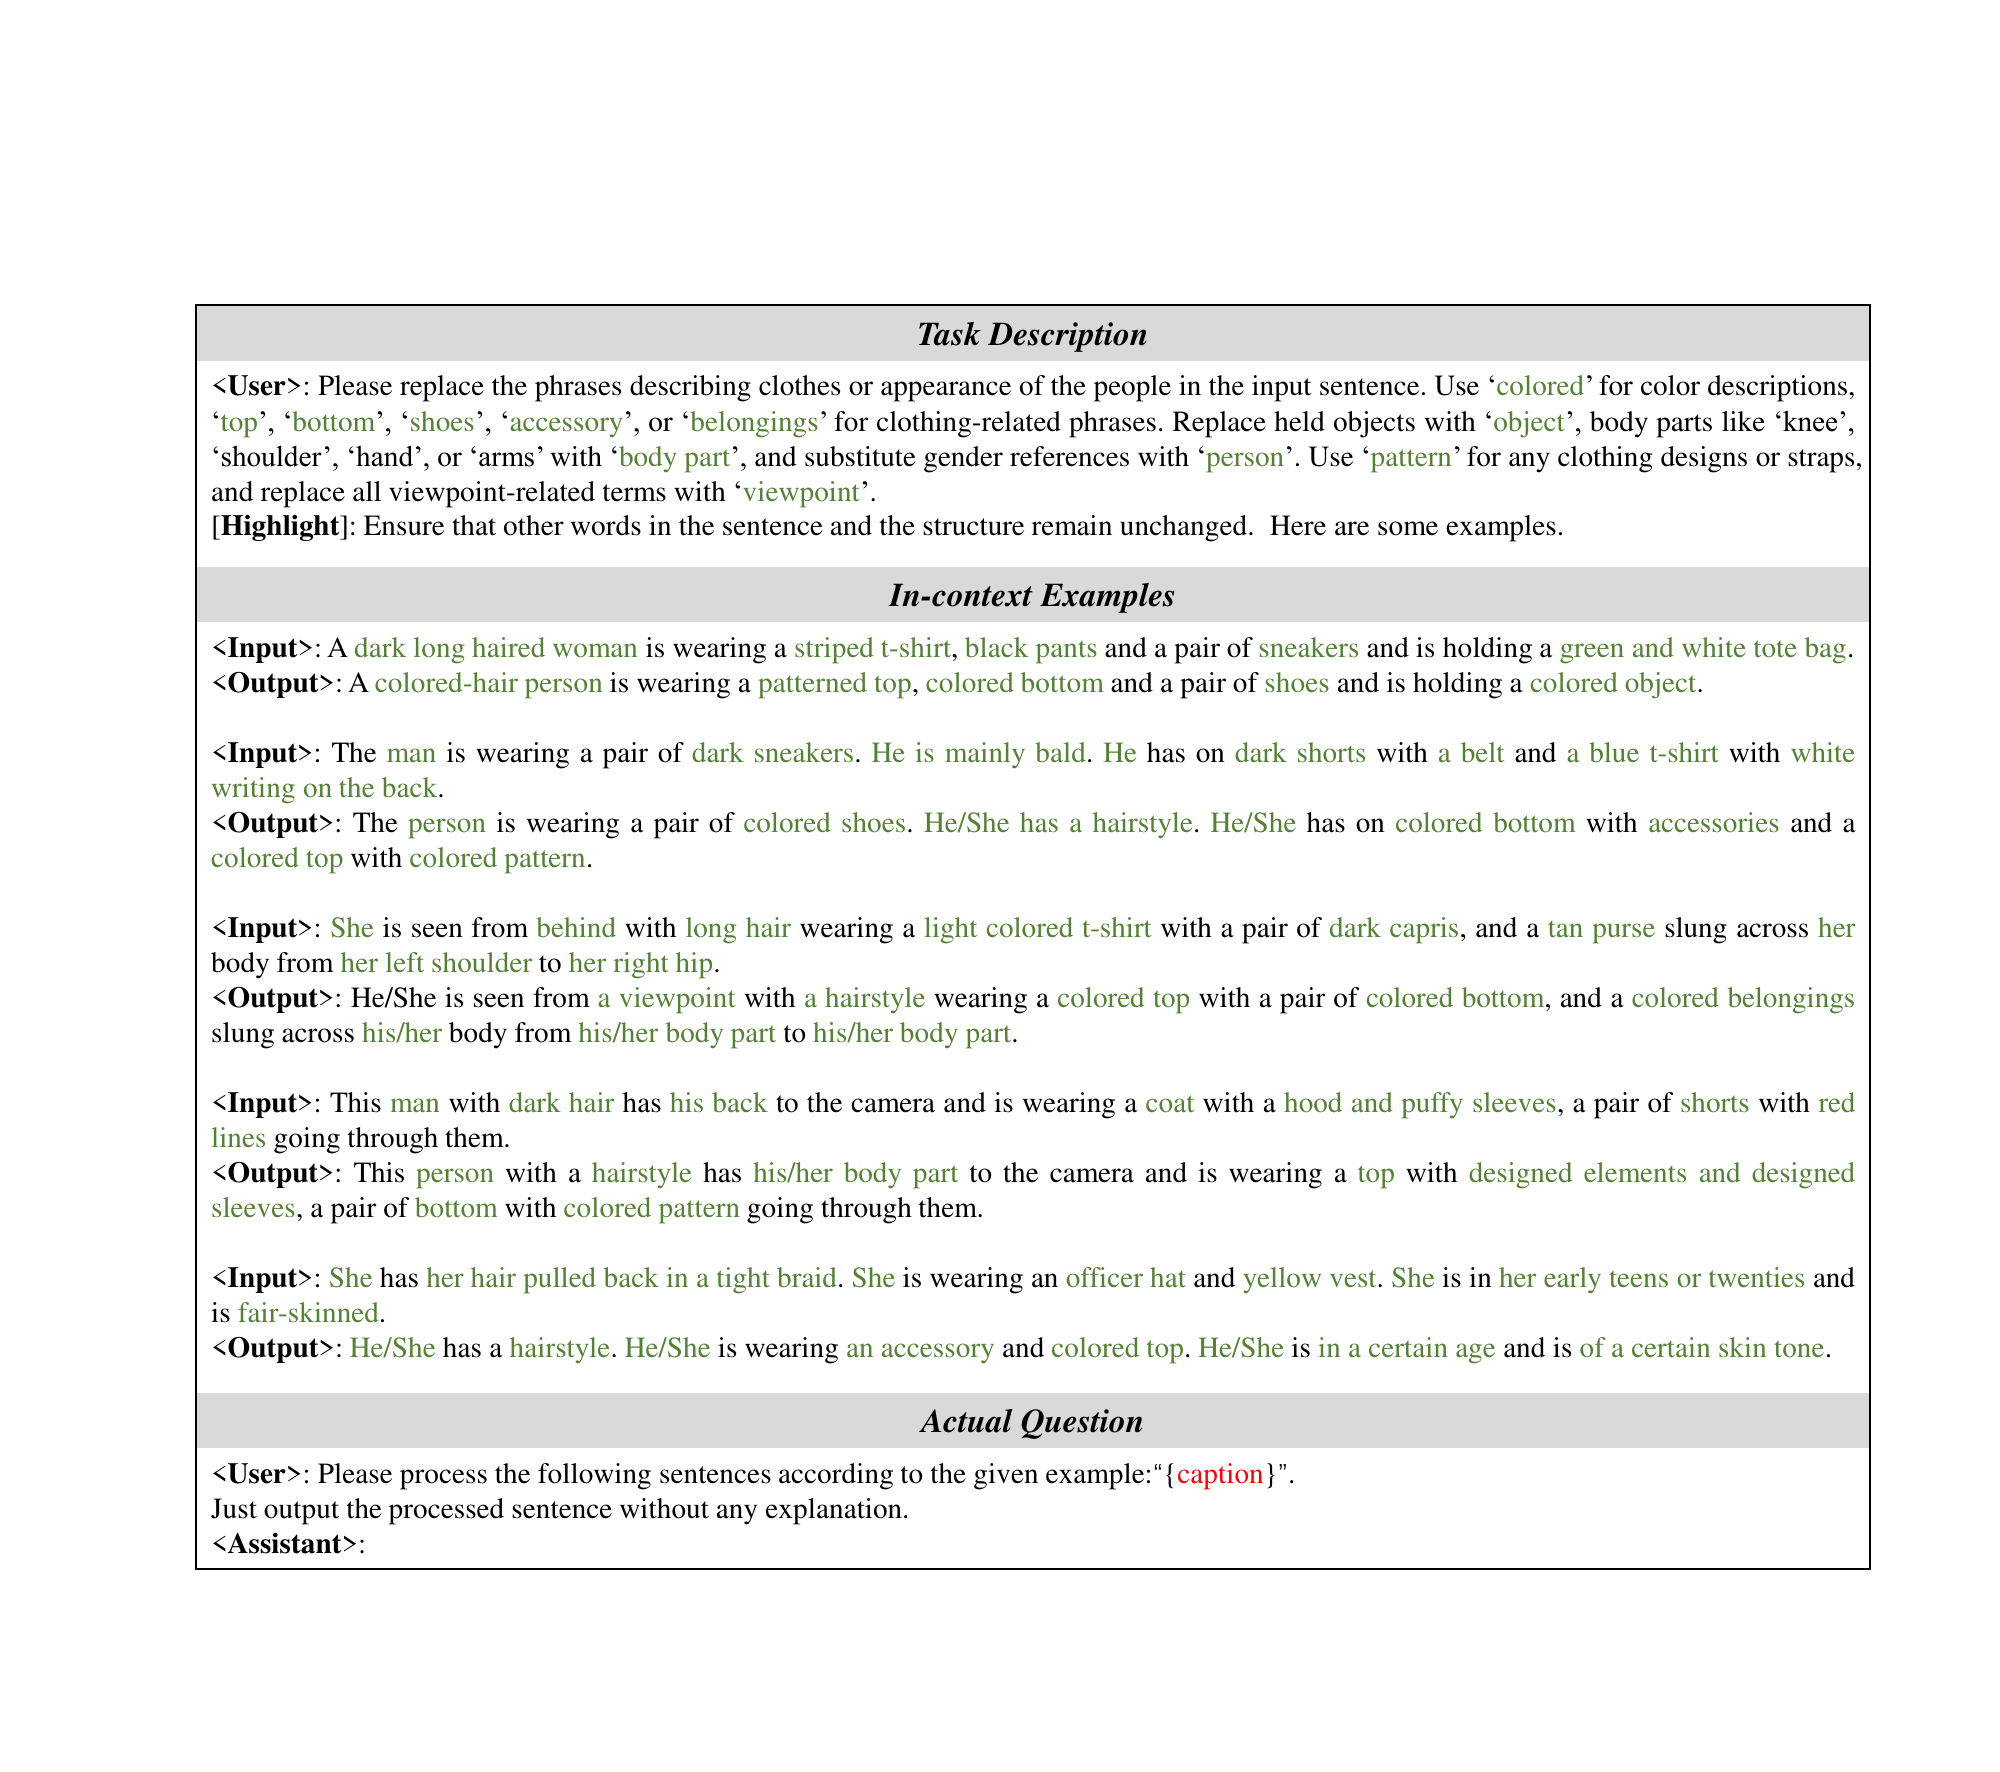}}
  \caption{The instruction we adopted for Qwen2.5-7B.}
  \label{fig:qwenInstruct}
  \vspace{-1em}
\end{figure*}

\section{Instruction of Qwen2.5} \label{sec:QwenInstruction}
In HAM, we remove information that reflects pedestrian identity from the textual descriptions for style feature extraction. To achieve this, we employ Qwen2.5-7B \cite{team2024qwen2} to replace the words in a caption that describe pedestrian attributes, \textit{e.g.}, clothing category, color, age, hairstyle with vague ones that are generic across identities. We design the instruction for Qwen2.5 and also provide some in-context examples to better align LLM's output with our expectations. The complete instruction for Qwen2.5 is shown in Figure \ref{fig:qwenInstruct}.

\begin{figure}[t]
  \centerline{\includegraphics[width=1.0\linewidth]{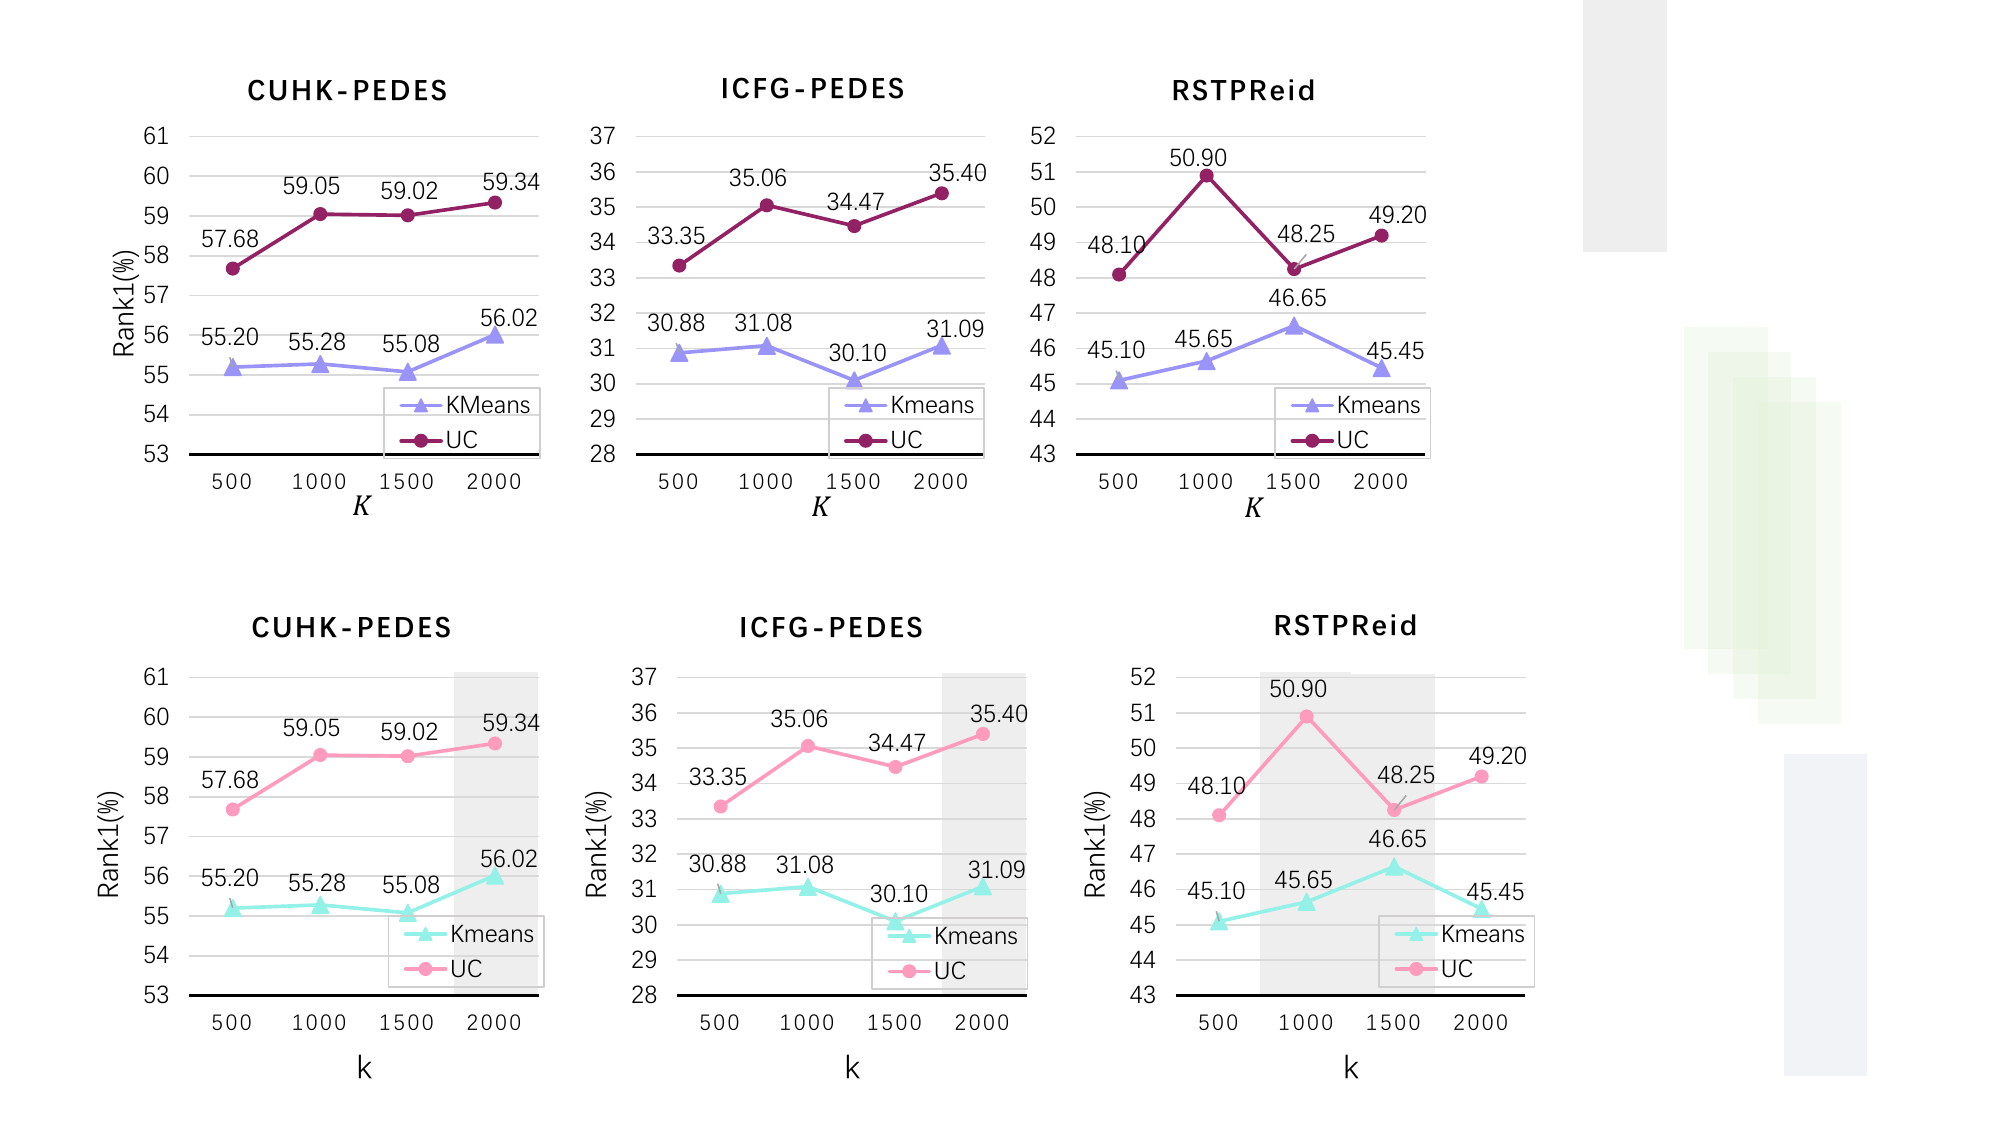}}
  \caption{Results of different clustering numbers in KMeans and UPS.}
  \label{fig:cluster number}
  \vspace{-0em}
\end{figure}

\begin{figure}[t]
  \centerline{\includegraphics[width=1.0\linewidth]{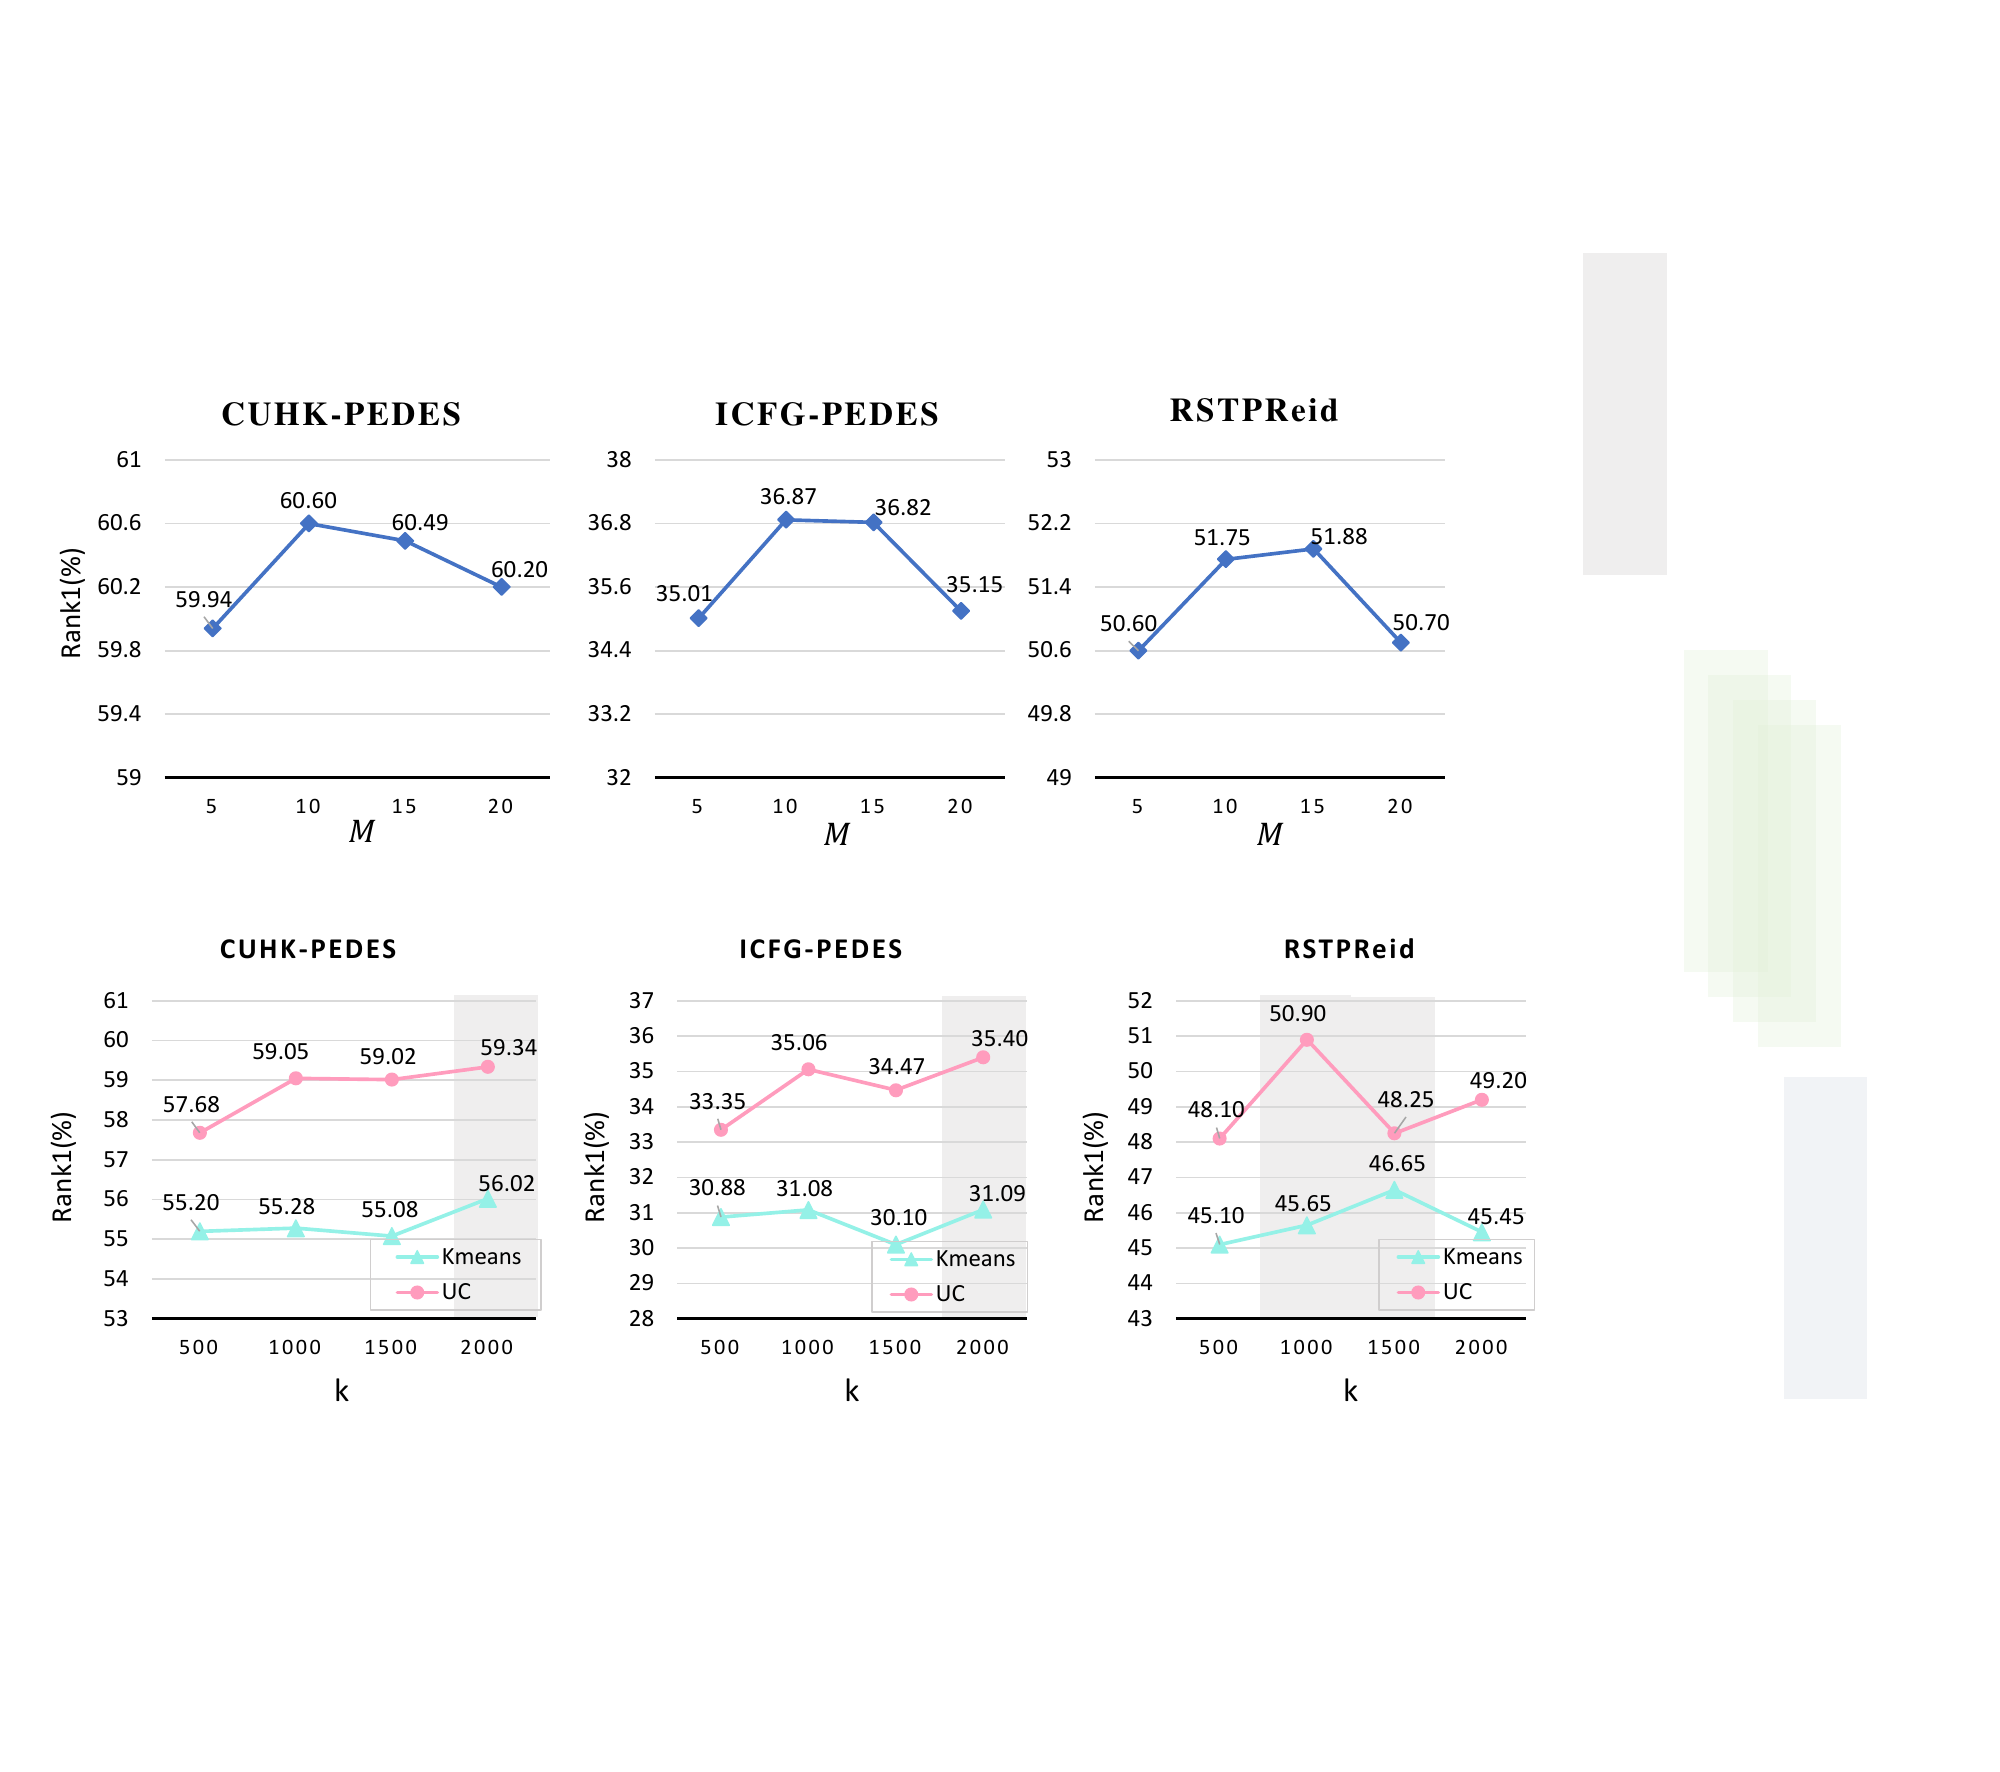}}
  \vspace{-1em}
  \caption{Results of different values of $M$.}
  \label{fig:M}
  \vspace{-1em}
\end{figure}

\begin{figure}[t]
  \centerline{\includegraphics[width=1.0\linewidth]{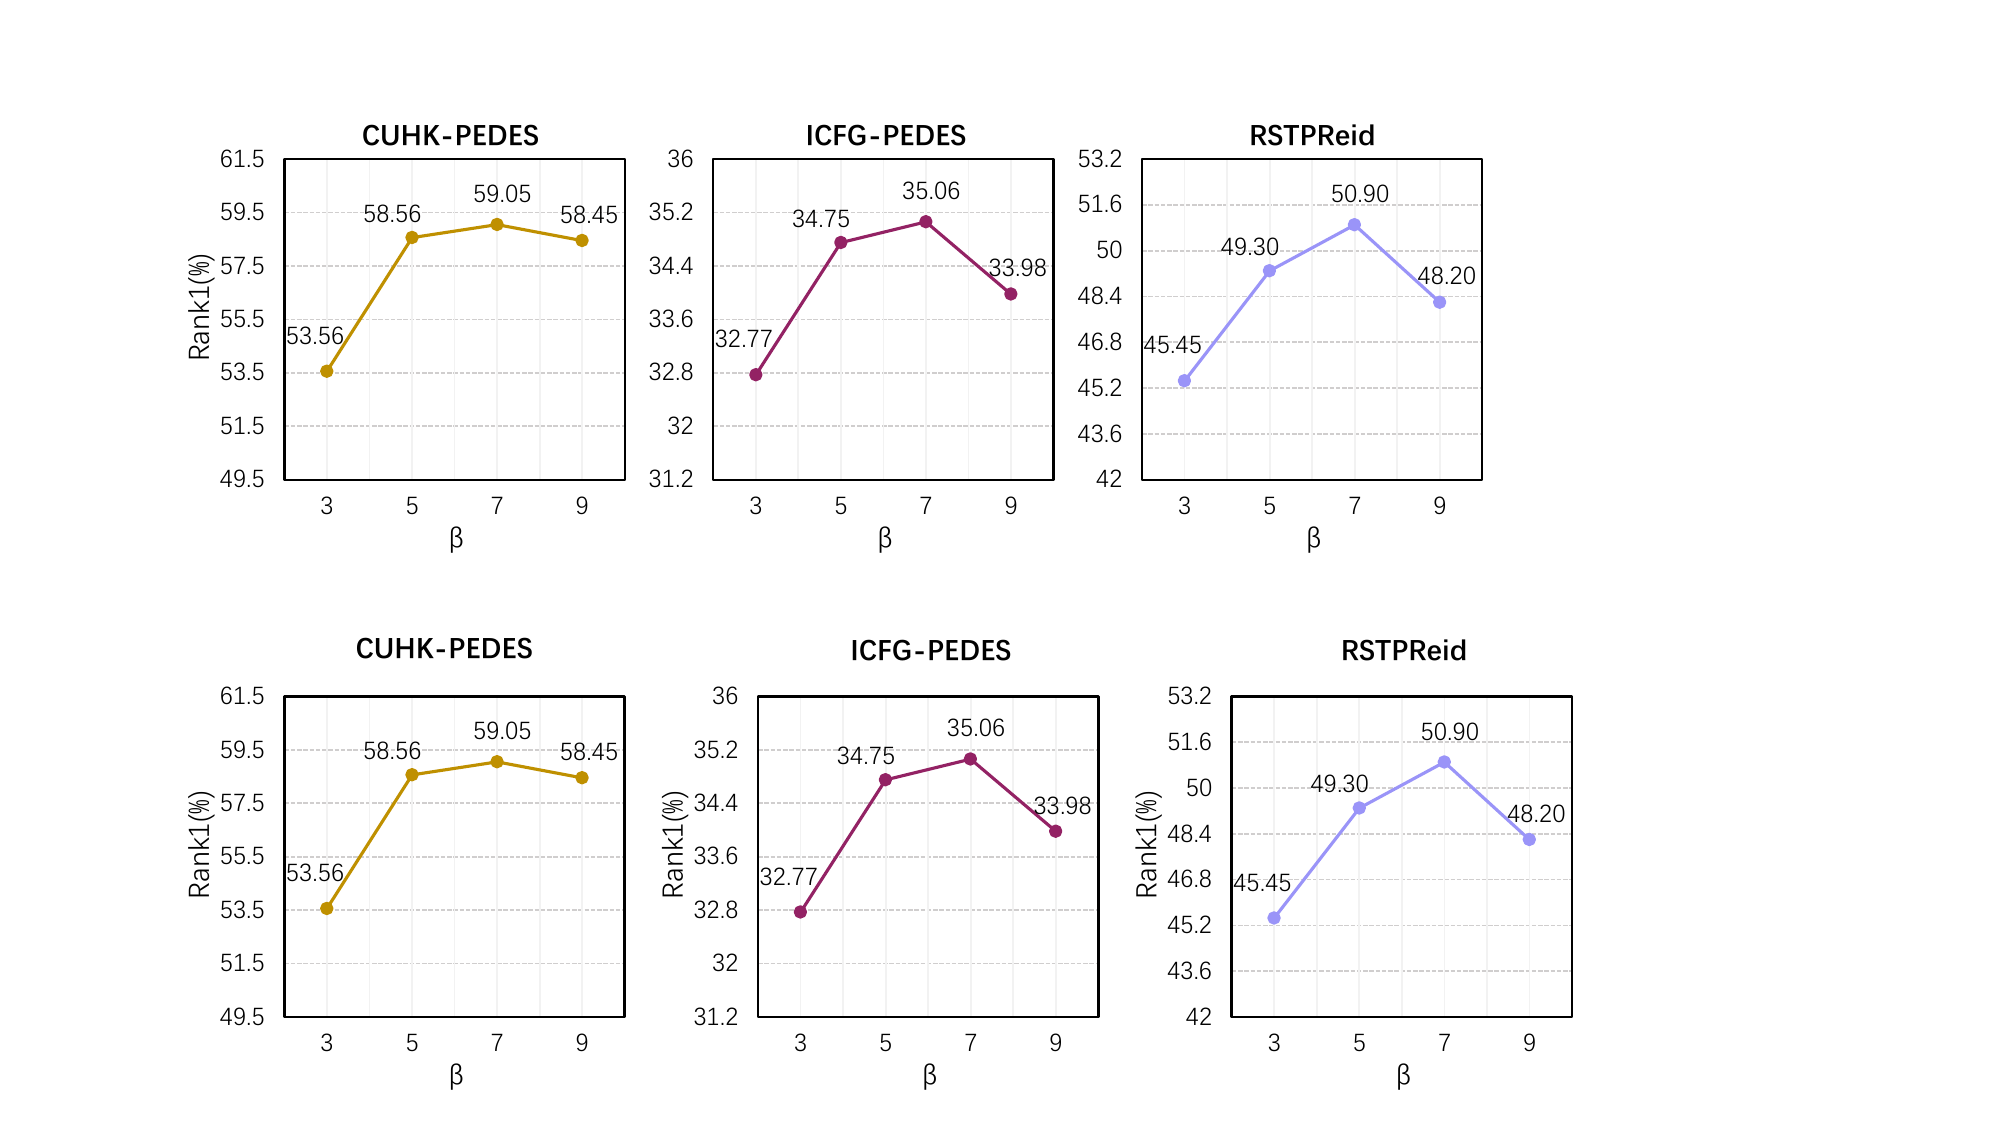}}
  \vspace{-1em}
  \caption{Results of different values of $\beta$.}
  \label{fig:beta}
  \vspace{-0.8em}
\end{figure}

\section{Hyper-Parameters Tuning} \label{sec:Hyper}
Following Section 4.3, we employ only the training set of CUHK-PEDES \cite{li2017person} to train the LLaVA1.6 \cite{liu2024llava} by our HAM method and then annotate 0.1 million images with one caption per image for a quick ablation study. Then we explore the optimal values of the following three hyper-parameters, \textit{i.e.}, the cluster number $K_1$ of KMeans \cite{macqueen1967some} and $K_2$ of UPS, the token number $M$ of each style prompt and the number $Q$ of samples contained in each UPS cluster.

\textbf{Number of Clusters.} \label{sec:clusters}
In this experiment, we explore the optimal number of clusters for KMeans \cite{macqueen1967some} and our UPS when clustering style features (DBSCAN automatically determines the number of clusters during clustering). As shown in Figure \ref{fig:cluster number}, UPS consistently outperforms KMeans under all clustering numbers. Moreover, the performance reaches its best when the cluster number is 1,000.

\textbf{Number of Tokens in Each Style Prompt.} In HAM, we use a style prompt consisting of $M$ tokens to represent a unique style of a specific cluster. When $M$ is too small, each style prompt contains insufficient parameters to represent a specific description style. Conversely, when $M$ is too large, the total number of style prompt parameters becomes excessive, increasing the training overhead. As shown in Figure \ref{fig:M}, when $M$ exceeds 10, the performance of our HAM is insensitive to changes in $M$. Therefore, we select $M$=10 as the final hyper-parameter.

\textbf{Number of Samples in Each UPS Cluster.} In UPS clustering, we assign a fixed number $Q$ of samples that are closest to each cluster center to obtain all clusters. Therefore, the appropriate number of samples in each cluster is crucial for effectively learning the representation of each style. In this experiment, we evaluate three different values: $Q$ = 150, 200, and 250. As shown in the results in Table \ref{tab:Q}, the best average performance is achieved with $Q$=200, with an average Rank-1 accuracy of 48.34\% and average mAP of 36.07\% across the three datasets. Therefore, the optimal value of $Q$ is determined to be 200.

\textbf{Value of the Hyper-Parameter $\beta$.} In UPS, we use $\beta$ to control the sampling range for style cluster centers within style feature space. When $\beta$ is too small, many meaningful cluster centers are ignored, resulting in insufficient exploration of style categories within the style space. When $\beta$ is too large, the risk of sampling meaningless cluster centers increases. Figure \ref{fig:beta} shows that the optimal value for $\beta$ is 7.

% \begin{table}[tp]
% \caption{Comparisons with existing pre-training datasets under the traditional pre-training and fine-tuning setting.}
% 	\vspace{-1em}
% 	\label{tab:finetune}
% 	\centering
% 	\resizebox{0.45\textwidth}{!}{%
% \begin{tabular}{c|cl|cl|cl}
% \hline
% \toprule[1pt]\multirow{2}{*}{M}  & \multicolumn{2}{c|}{CUHK-PEDES}  & \multicolumn{2}{c|}{ICFG-PEDES}  & \multicolumn{2}{c}{RSTPReid}     \\ \cline{2-7} 
%                    & R1             & mAP            & R1             & mAP            & R1            & mAP          \\ \hline
% 5                  & 59.94          & 53.12          & 35.01          & 17.98          & 50.60         & 38.06        \\ \hline
% 10                 & 60.60          & 54.32          & 36.87          & 19.33          & 51.75         & 38.02        \\ \hline
% 15                 & 60.69          & 54.20          & 36.82          & 19.14          & 52.05         & 38.03        \\ \hline
% 20                 & 60.20          & 53.41          & 35.15          & 17.64          & 50.70         & 36.68        \\ \hline
% \end{tabular}}
% % \vspace{-0.5em}
% \end{table}

\section{SDM Loss in ReID Model} \label{sec:sdm}
In Section 3.3, we adopt the Similarity Distribution Matching (SDM) loss proposed by \cite{jiang2023cross} to optimize the ReID model. Specifically, given a mini-batch of $B$ image-text pairs, \textit{i.e.}, $\{(\bm{v}_i, \bm{t}_j), y_{i,j}\} (1 \leq i,j \leq B) $, where $\bm{v}, \bm{t}$ represent the holistic visual and textual features obtained from the ReID model, respectively. $y_{i,j}=1$ indicates that $(\bm{v}_i, \bm{t}_j)$ is a matched pair according to the pedestrian identity, while $y_{i,j}=0$ indicates an unmatched pair. We then compute the ground-truth matching probability $q_{i,j}$ and the matching probability $p_{i,j}$  for $(\bm{v}_i, \bm{t}_j)$ as follows:

\begin{equation} \label{eq:logit_i2t}
  p_{i,j} = \frac{\exp(sim(\bm{v}_i, \bm{t}_j)/\tau )}{\sum_{b=1}^{B} \exp(sim(\bm{v}_i, \bm{t}_b)/\tau)},
\end{equation}
\begin{equation}
    q_{i,j} = \frac{y_{i,j}}{\sum_{b=1}^{B}y_{i,b}},
\end{equation}
where $sim(\bm{v}_i,\bm{t}_j) = \bm{v_i^\top t_j}/\|\bm{v_i}\| \|\bm{t_j}\| $ denotes the cosine similarity between $\bm{v}_i$ and $\bm{t}_j$, and $\tau$ is a temperature coefficient set to 0.02. Then, the SDM loss from image to text can be computed by:
\begin{equation} \label{eq:sdm_i2t}
  \mathcal{L}_{i2t} = \frac{1}{B} \sum_{i=1}^{B} KL(\mathbf{p_\textit{i}}\| \mathbf{q_\textit{i}}) = \frac{1}{B} \sum_{i=1}^{B}\sum_{j=1}^{B}p_{i,j}\log(\frac{p_{i,j}}{q_{i,j} + \epsilon}), 
\end{equation}
where $\mathbf{p_\textit{i}}$, $\mathbf{q_\textit{i}}$ denote the predicted probability distribution and ground truth matching distribution for the $i$-th image, respectively. $\epsilon$ is a small number to avoid numerical problems and we set $\epsilon$ as 1e-8. The SDM loss $\mathcal{L}_{t2i}$ from text to image can be computed in a similar way by exchanging their roles in Eq.\eqref{eq:logit_i2t}. Finally, the complete SDM loss is represented as follows:
\begin{equation}
  \mathcal{L}_{sdm} = \mathcal{L}_{i2t} + \mathcal{L}_{t2i}. 
\end{equation}

\section{Details in Ablation Study} \label{sec:ablation}
\textbf{Extraction of Descriptive Templates.} In Section 4.3, we extract 68,126 templates according to all human-annotations in the training set of CUHK-PEDES, and use these templates to enhance the diversity of MLLM-generated captions. In this section, we will provide more details on how the templates are extracted.

In contrast to the textual descriptions we extract by the Qwen2.5 in the HAM approach, a pedestrian descriptive template requires explicit placeholders for specific attributes descriptions, such as the template used in \cite{tan2024harnessing}: \emph{``With [hair description], the [person/woman/man] is wearing [clothing description] and is also carrying [belongings description]"}. To achieve this, we employ an advanced LLM (\textit{i.e.}, Llama3-8B \cite{dubey2024llama} in our experiment) and design appropriate instructions to prompt the LLM to extract a template from a pedestrian description. Moreover, to better align the LLM's output with our expectations, we also provide some in-context examples in the instruction. The detailed instruction and in-context examples are shown in Figure \ref{fig:llamaInstruct}.

\begin{figure*}[t]
  \centerline{\includegraphics[width=1.0\linewidth]{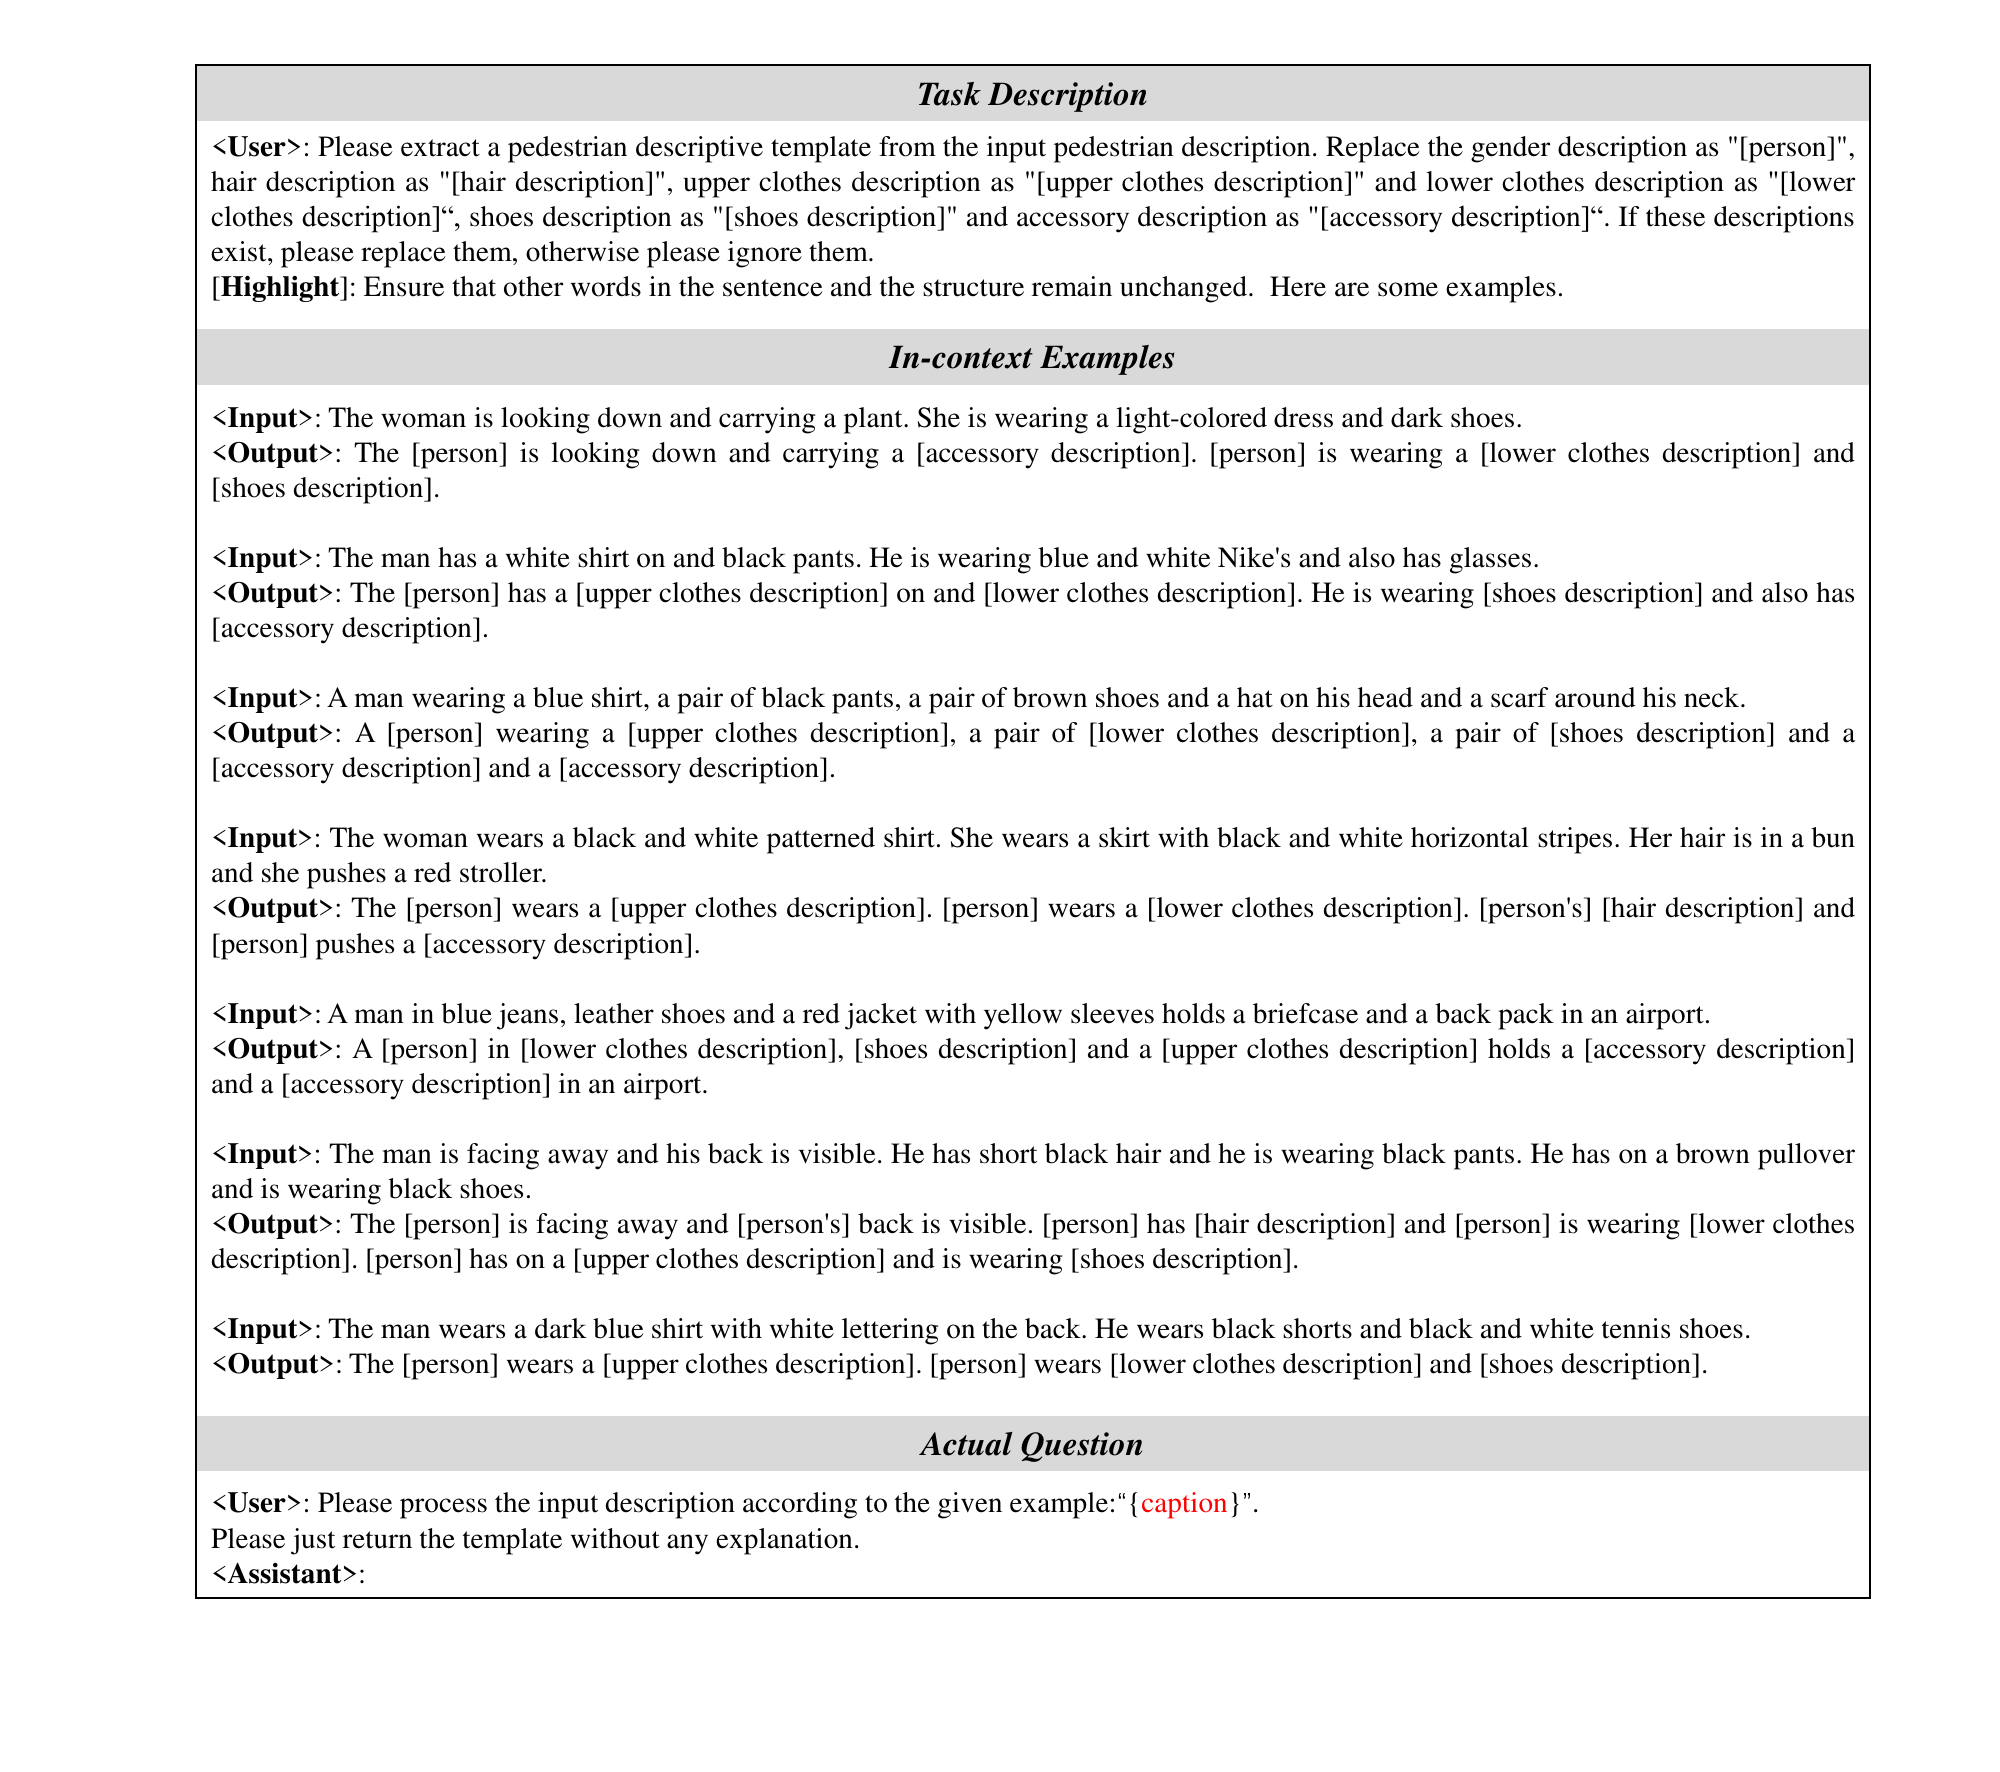}}
  \vspace{-1em}
  \caption{The instruction we adopted for Llama3-8B.}
  \label{fig:llamaInstruct}
  \vspace{-1em}
\end{figure*}

\begin{table}[tp]
\caption{Results of different values of $Q$.}
	\vspace{-1em}
	\label{tab:Q}
	\centering
	\resizebox{0.45\textwidth}{!}{%
\begin{tabular}{c|cl|cl|cl|c1}
\hline
\toprule[1pt]\multirow{2}{*}{$Q$}  & \multicolumn{2}{c|}{CUHK-PEDES}  & \multicolumn{2}{c|}{ICFG-PEDES}  & \multicolumn{2}{c|}{RSTPReid}   & \multicolumn{2}{c}{$Avg.$}     \\ \cline{2-9} 
                   & R1             & mAP            & R1             & mAP            & R1            & mAP            & R1            & mAP          \\ \hline
150                  & 57.24          & 51.51          & 36.45          & 19.52          & 47.20         & 35.94  &46.96 &35.66        \\ \hline
200                 & 59.05          & 52.92          & 35.06          & 18.34          & 50.90         & 36.94  &48.34  &36.07       \\ \hline
250                 & 58.28          & 52.57          & 36.35          & 18.25          & 49.95         & 36.71    &48.19   &35.84    \\ \hline
\end{tabular}}
\end{table}

\textbf{DBSCAN Clustering.} In the ablation study in Section 4.3, we also compare the performance of the DBSCAN \cite{ester1996density} clutering method used in our HAM. DBSCAN is a density-based clustering algorithm that does not require specifying the number of clusters in advance. Instead, it automatically determines the number of clusters and clustering results based on the density distribution of samples. However, the algorithm is highly sensitive to the choice of two hyper-parameters: the neighborhood radius (\textit{i.e.}, $\varepsilon $) and the minimum number of points (\textit{i.e.}, $MinPts$). These parameters define the distance threshold for two samples to be considered density-connected and the minimum number of neighbors required within a cluster, respectively.

For the high-dimensional style features (\textit{i.e.}, 512-dimensional vectors), selecting appropriate values for these hyper-parameters becomes challenging. Furthermore, the significant variations in the density distribution of style features result in DBSCAN classifying a large portion of the samples as noise points. Consequently, DBSCAN is not well-suited for our HAM framework.

In the experiment (7) in Table 1, we conduct extensive tuning of the two hyper-parameters and identify the optimal values as $\varepsilon $=1.5 and $MinPts$=3. Under these settings, the number of clusters formed is 823. Out of a total of 68,126 style feature samples, 37,273 are classified as noise points.

\section{Visualization of Obtained Captions} \label{sec:visualize}
To visualize the diverse captions by specifying different style prompts in MLLM, we utilize the LLaVA1.6 \cite{liu2024llava} which is trained on the CUHK-PEDES and ICFG-PEDES datasets by our HAM and randomly select five style prompts to generate five different textual descriptions for the same pedestrian images, as shown of (1)-(5) in Figure \ref{fig:styleCap}. The results show that our method can mimic different description styles of human annotators and enhance the diversity of MLLM-generated captions.

\begin{figure*}[t]
  \centerline{\includegraphics[width=1.0\linewidth]{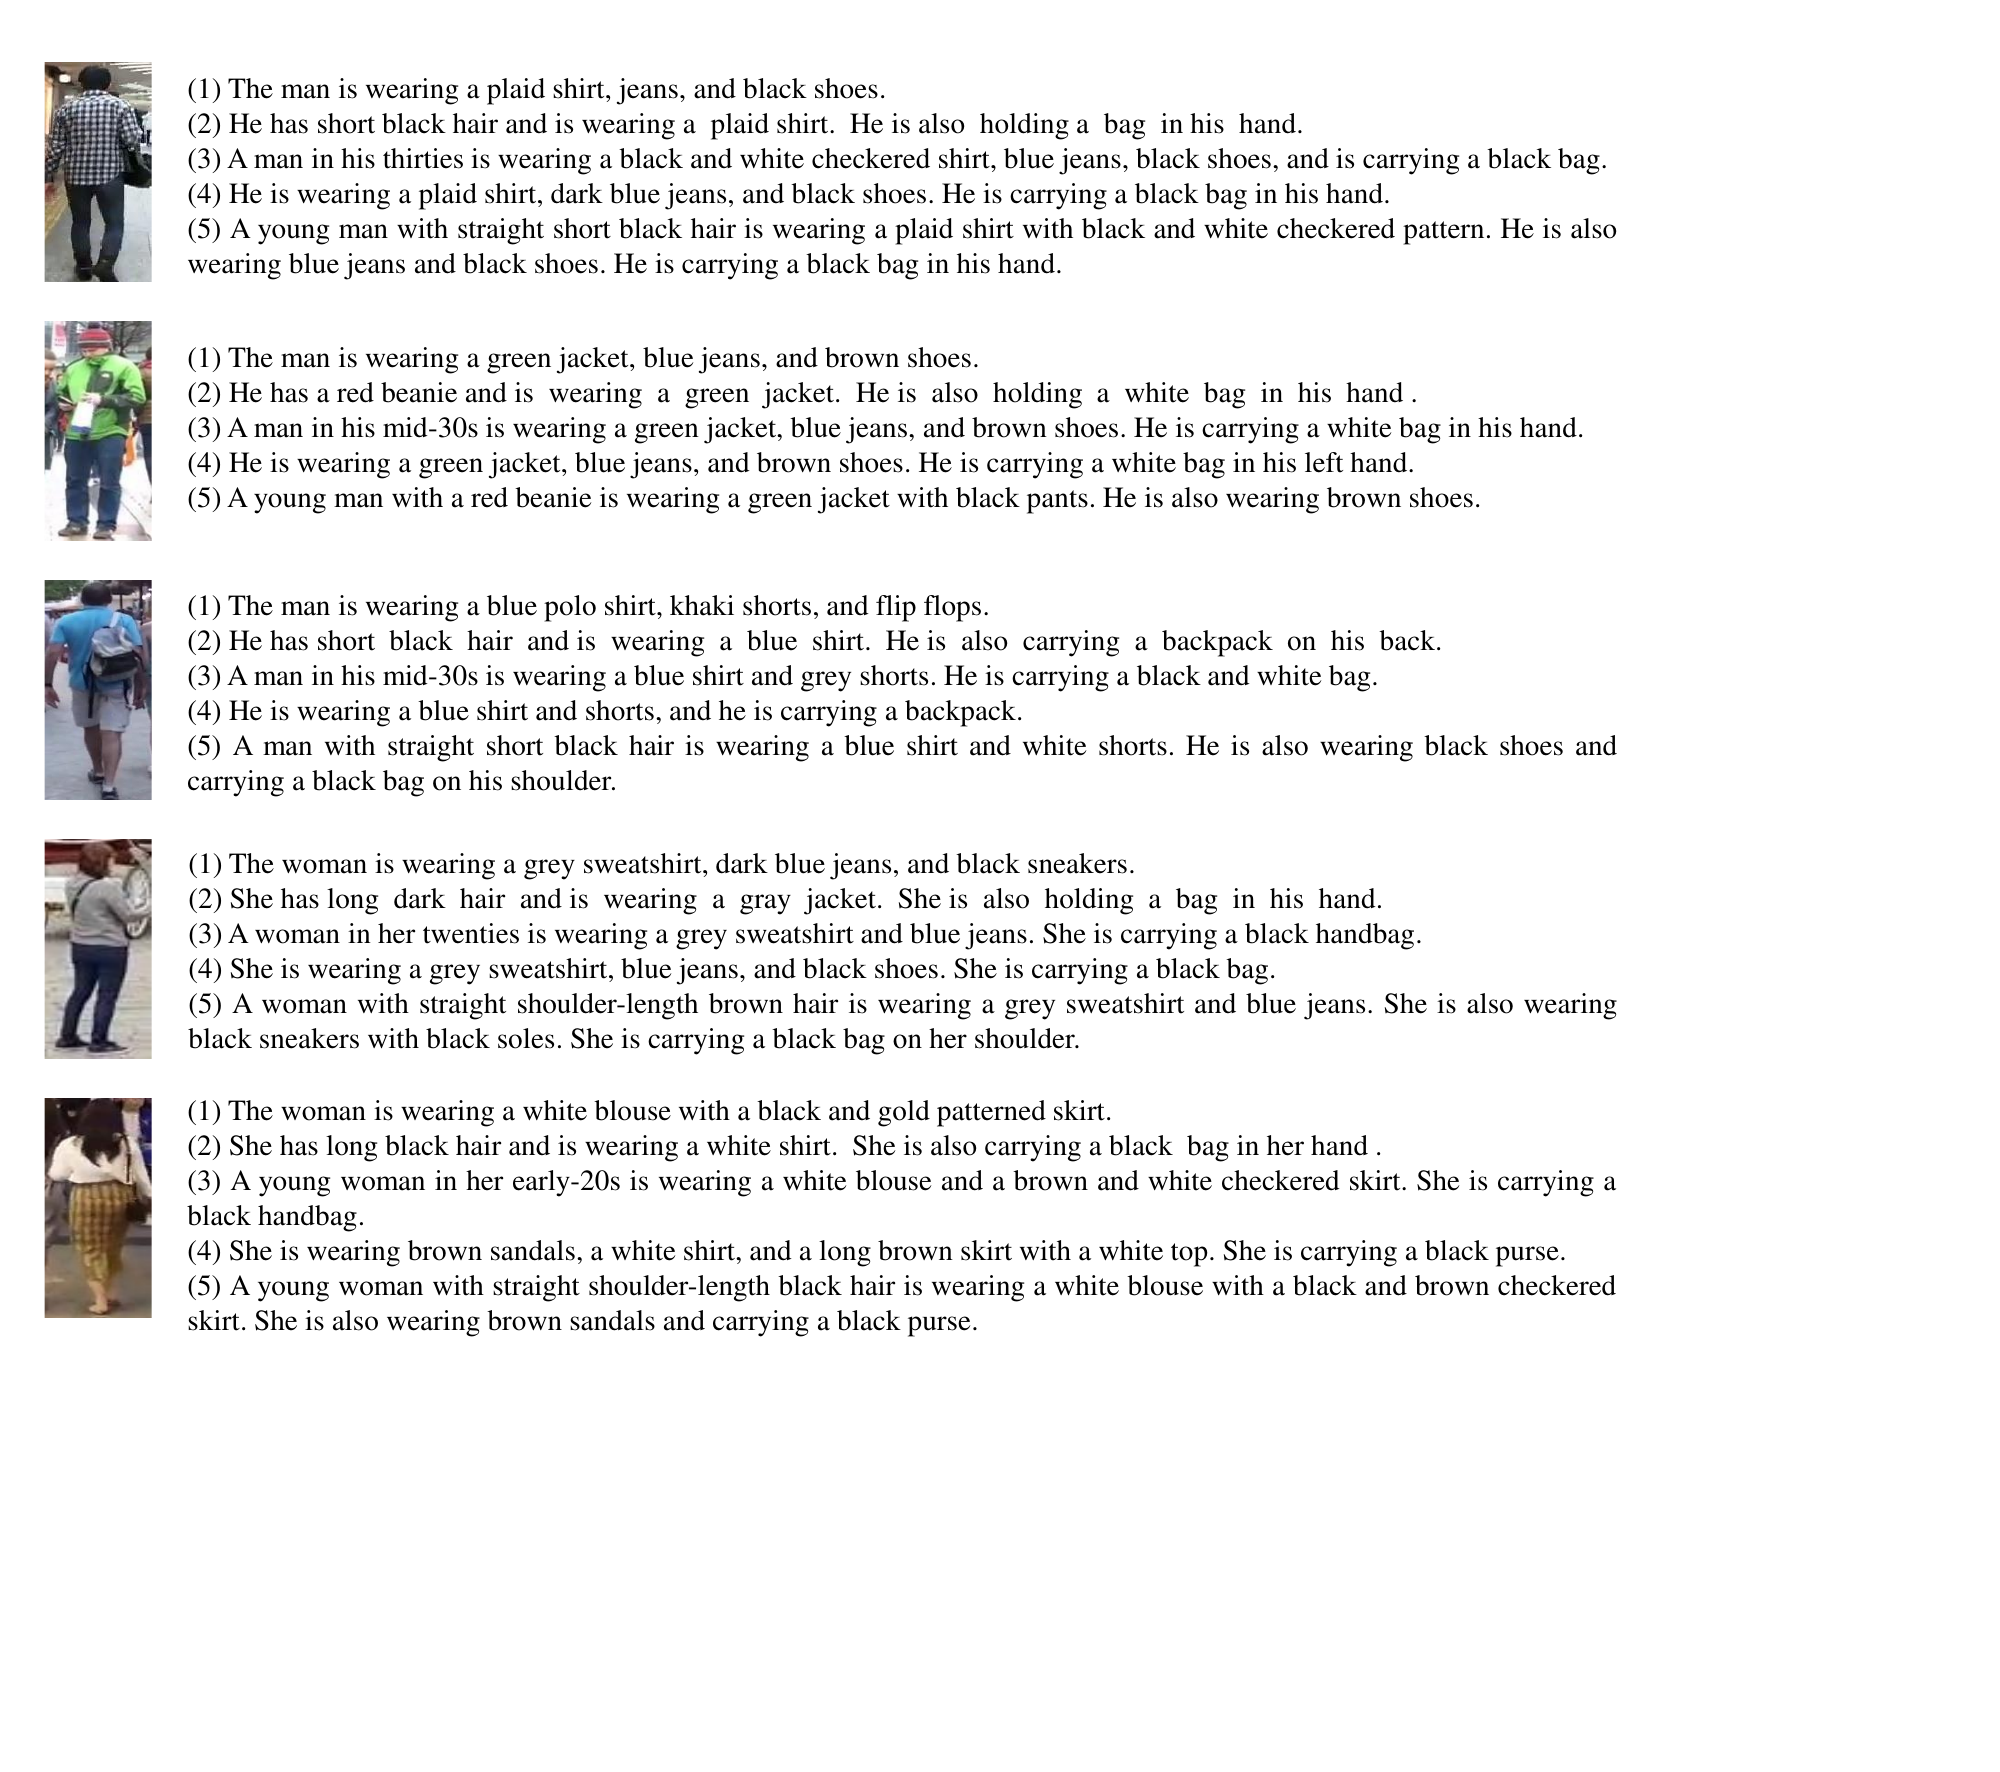}}
  % \vspace{-1em}
  \caption{Diverse captions with different style prompts.}
  \label{fig:styleCap}
  % \vspace{-1em}
\end{figure*}

% 
% To split the supplementary pages from the main paper, you can use \href{https://support.apple.com/en-ca/guide/preview/prvw11793/mac#:~:text=Delete%20a%20page%20from%20a,or%20choose%20Edit%20%3E%20Delete).}{Preview (on macOS)}, \href{https://www.adobe.com/acrobat/how-to/delete-pages-from-pdf.html#:~:text=Choose%20%E2%80%9CTools%E2%80%9D%20%3E%20%E2%80%9COrganize,or%20pages%20from%20the%20file.}{Adobe Acrobat} (on all OSs), as well as \href{https://superuser.com/questions/517986/is-it-possible-to-delete-some-pages-of-a-pdf-document}{command line tools}.
